# Supplementary material for: Static and Dynamic Robust PCA and Matrix Completion: A Review
Source: arXiv:1803.00651 source file (2018-05-25)
Supplement: Supplementary file 1 [file proc_appendix.tex]

\appendices
\section{Moving Object Model used for outlier support generation}
The Moving Object model is a practically motivated model that, in a video, simulates a person pacing back and forth in a room. It provides a simple way to ensure that the fraction of outliers per row are larger than that of the fraction of outliers per column. More details are provided at \cite[Model G.24]{rrpcp_dynrpca}.

\begin{sigmodel}[Moving Object Model]\label{mod:moving_object}
%\emph{Parameters}: $c_0$, $\tau$, $s$. %Consider a time interval of length $2\tau$ . Denote the support of sparse signal at time $t$ by $\mathcal{T}_t$. Define $\bbeta = \lceil c_0 \tau \rceil$. Then, for the first $\tau$ frames denoting downward motion, [Moving object model]
Let $\bbeta = \lceil c_0 \tau \rceil$. Assume that the $\T_t$ satisfies the following. For the first $\tau$ frames (downward motion),
\begin{align*}
\mathcal{T}_t = \begin{cases}
[1,\ s], &\ t \in [1, \beta] \\
[s+1,\ 2s], &\ t \in [\beta + 1, 2 \beta] \\
\vdots \\
[(1/c_0 - 1)s + 1,\ s/c_0], &\ t \in [\tau - \beta + 1, \tau] \\
\end{cases}
\end{align*}
for the next $\tau$ frames (upward motion),
\begin{align*}
\mathcal{T}_t = \begin{cases}
[(1/c_0 - 1)s + 1,\ s/c_0], &\ t \in [\tau + 1,\ \tau + \beta] \\
%[(1/c_0 - 2)s + 1,\ (1/c_0 - 1) s], &\ t \in [\tau + \beta + 1, \tau + 2\beta] \\
\vdots \\
[s+1,\ 2s] &\ t \in [2\tau - 2\beta + 1, 2\tau - \beta] \\
[1,\ s], &\ t \in [2\tau - \beta + 1, 2\tau]. \\
\end{cases}
\end{align*}
Starting at $t=2\tau+1$, the above pattern is repeated every $2\tau$ frames until the end, $t=\tmax$.
\end{sigmodel}
